# Supplementary material for: The End of Slow Networks: It's Time for a Redesign
Source: arXiv:1504.01048 source file (2015-12-19)

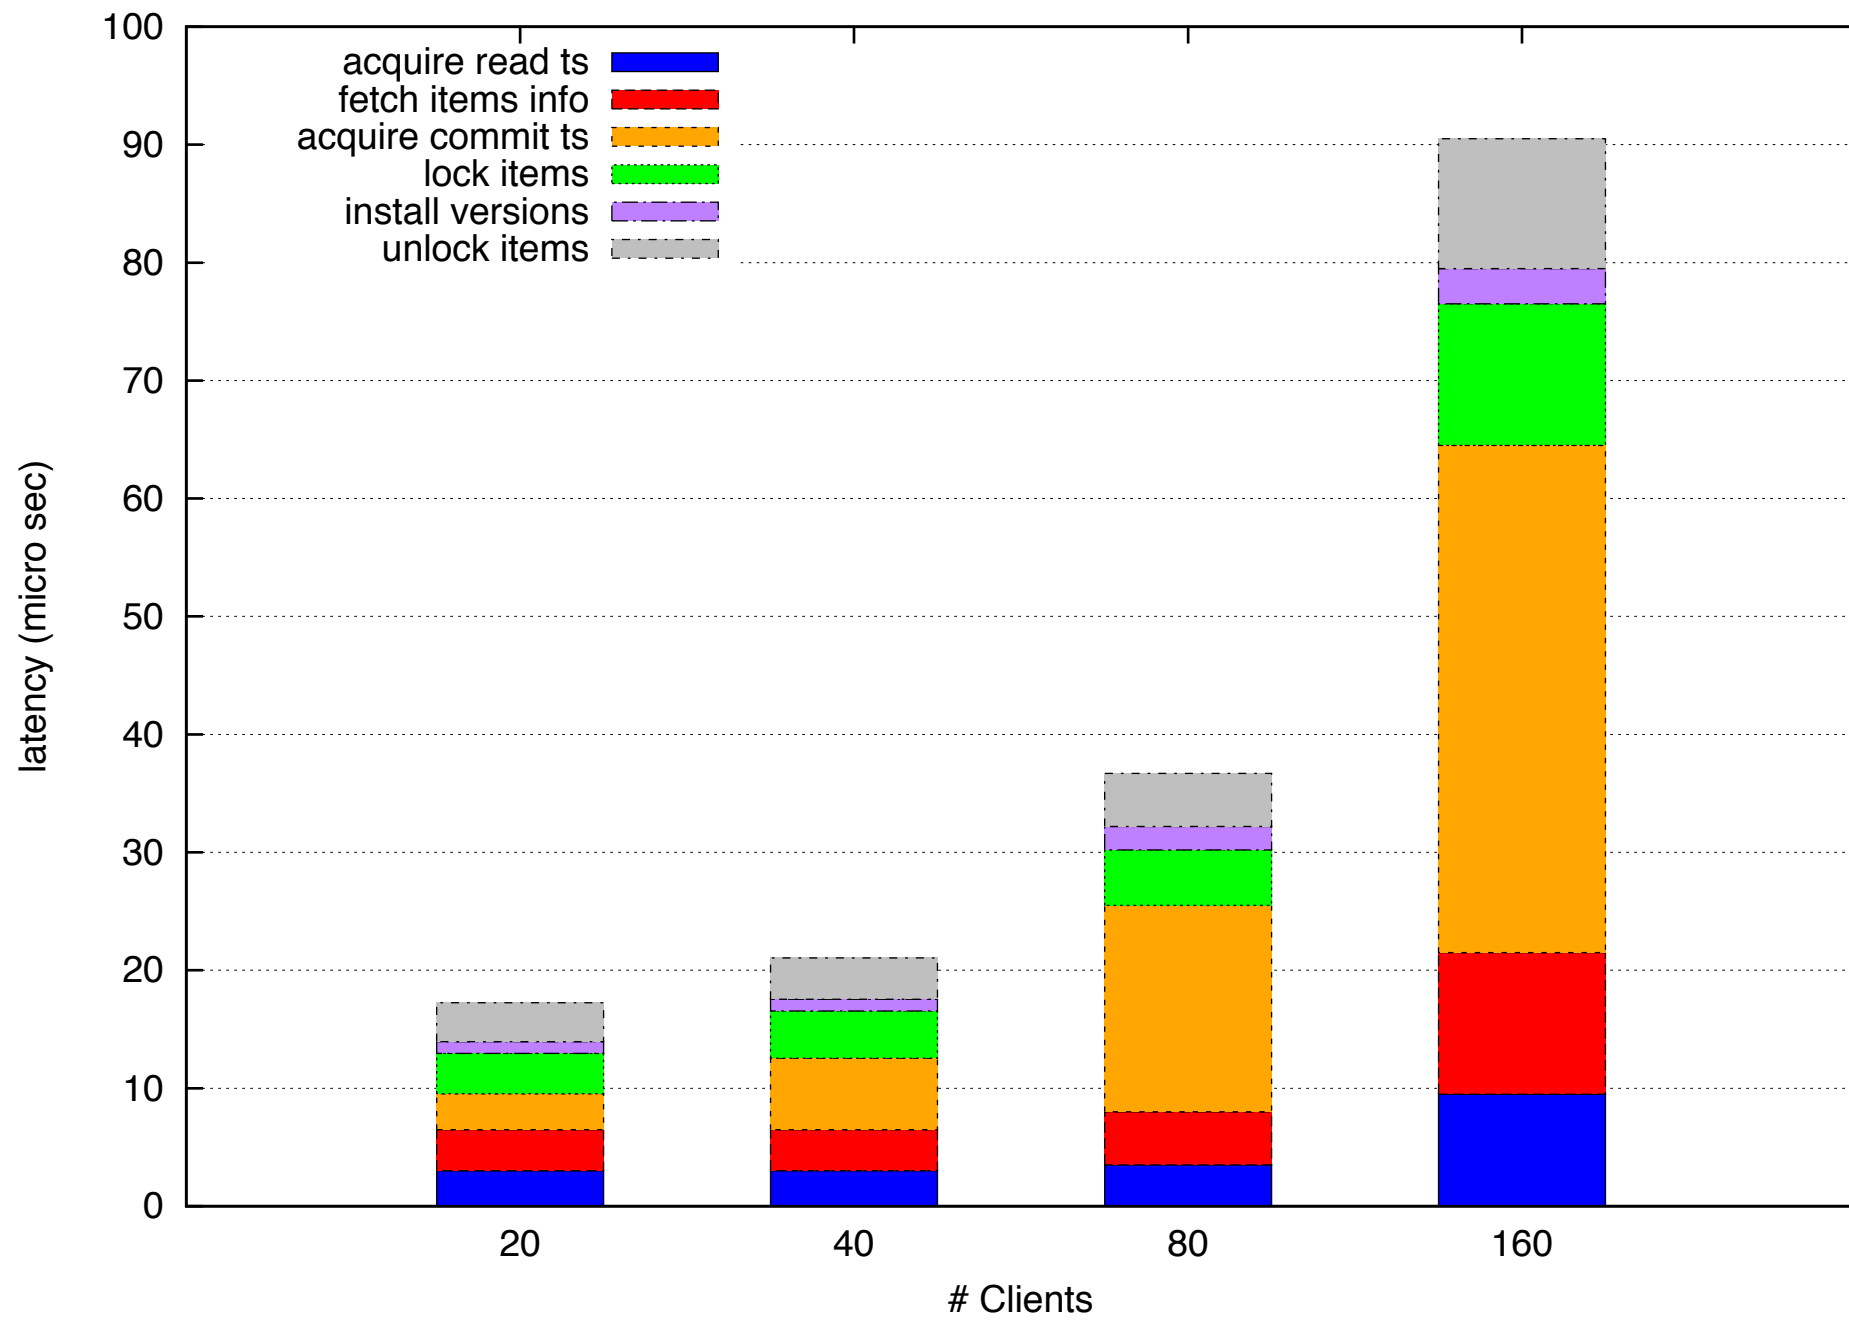

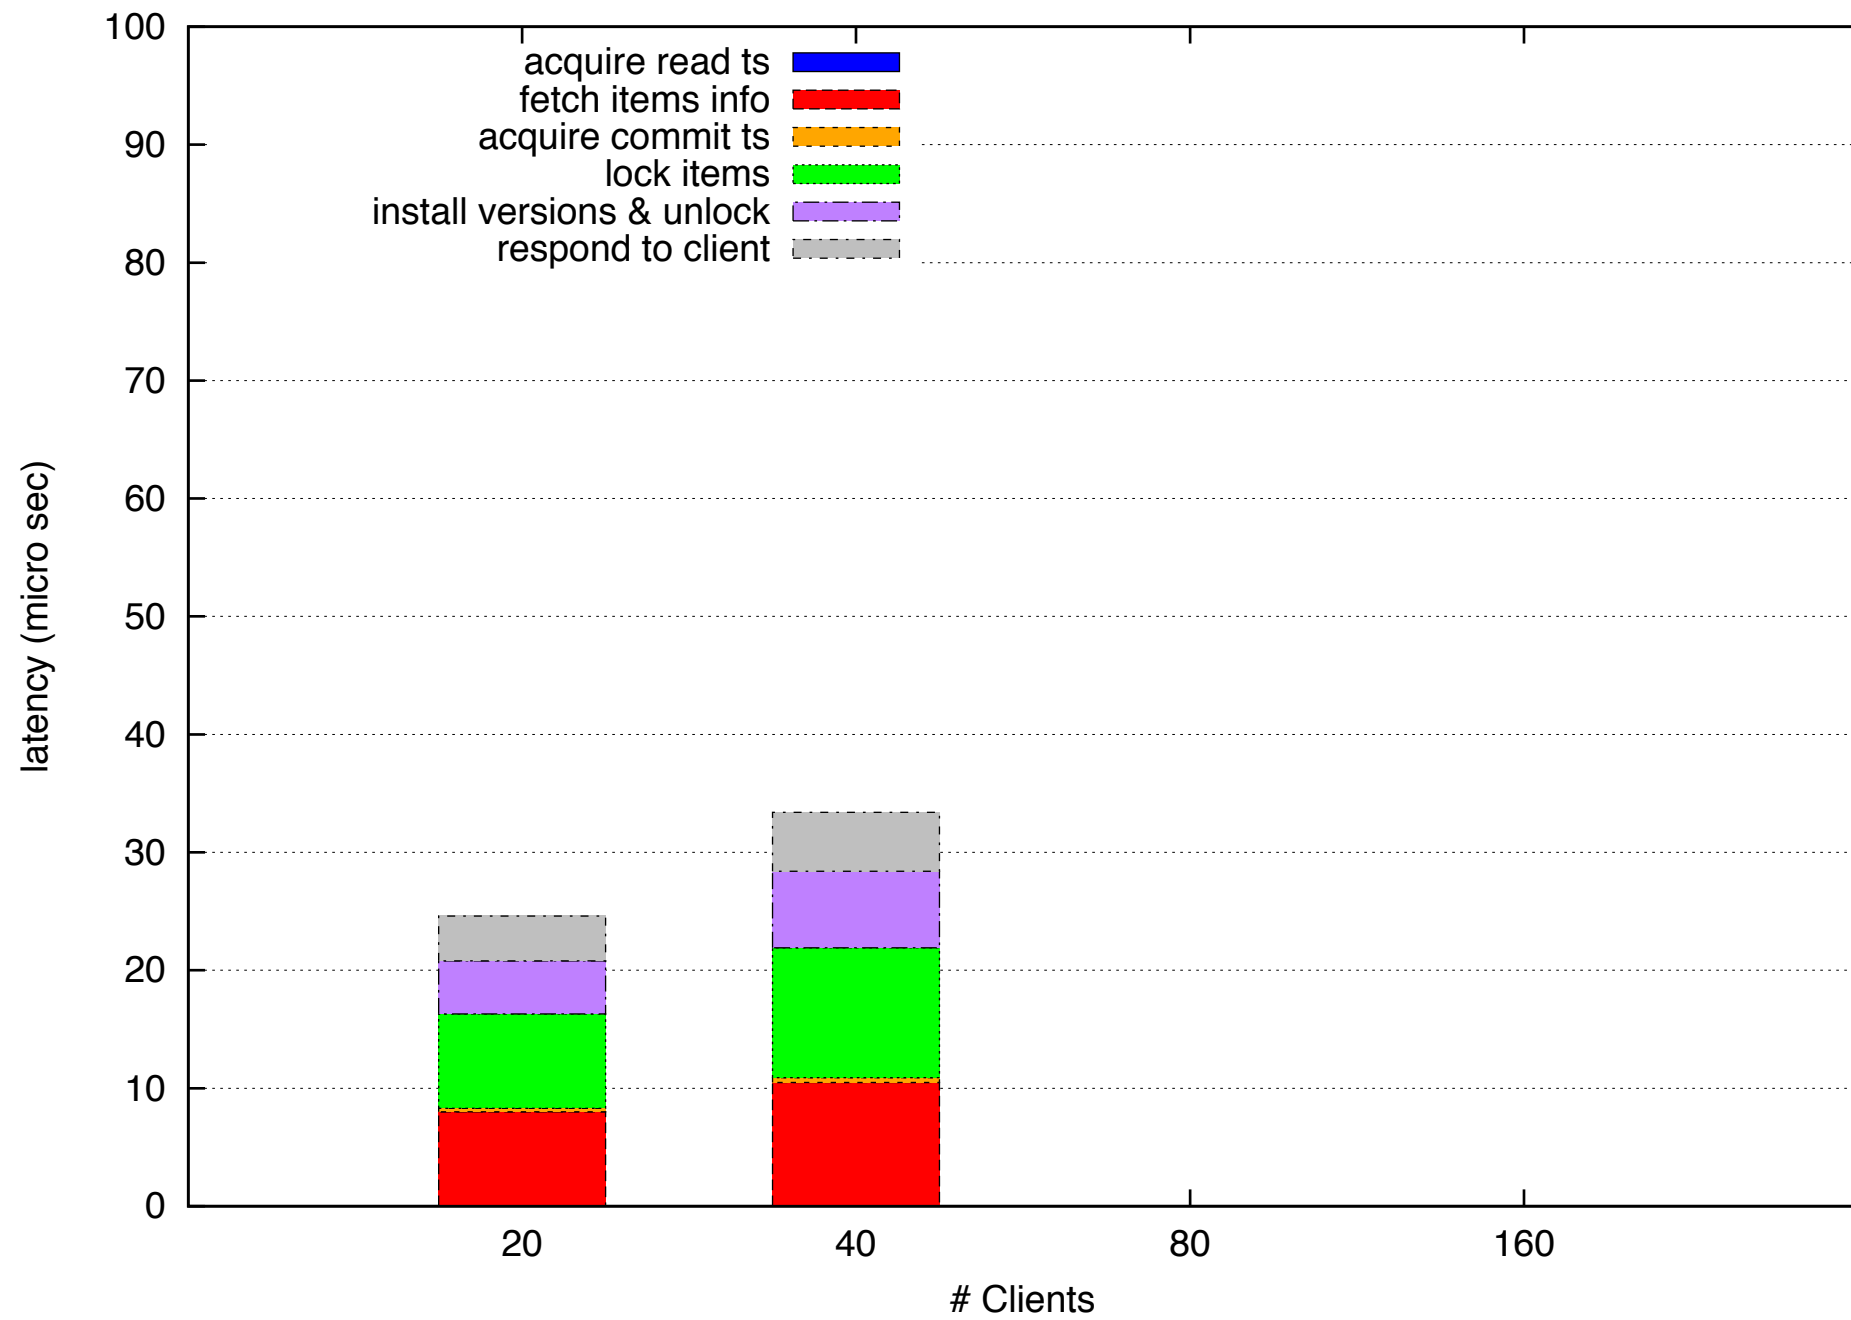

Supplement: Supplementary file 1 [file rdma-SI-latency-breakdown.pdf]
